# Supplementary material for: I-INR: Iterative Implicit Neural Representations
Source: arXiv:2504.17364 source file (2026-04-28)

PSNR: 17.52 dB

PSNR: 21.30 dB

PSNR: 24.88 dB **(+3.58)**

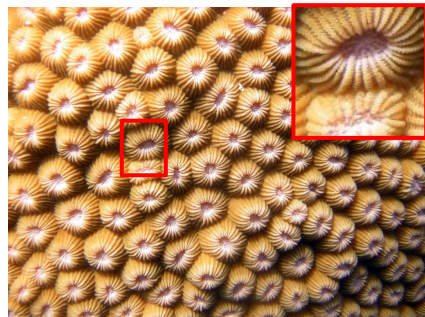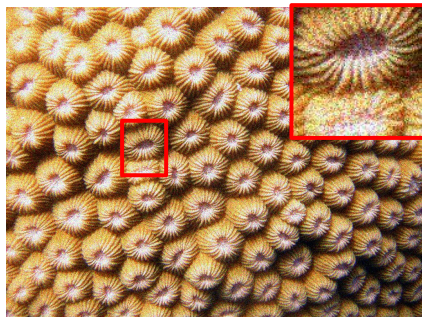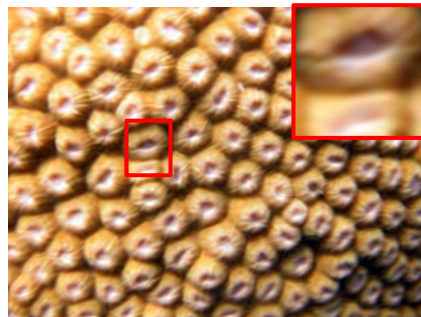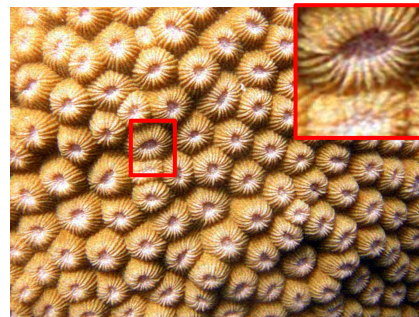

Ground Truth

Noisy

SIREN

Iterative-SIREN

PSNR: 21.84 dB

PSNR: 24.06 dB **(+2.22)**

PSNR: 22.52 dB

PSNR: 24.21 dB **(+1.69)**

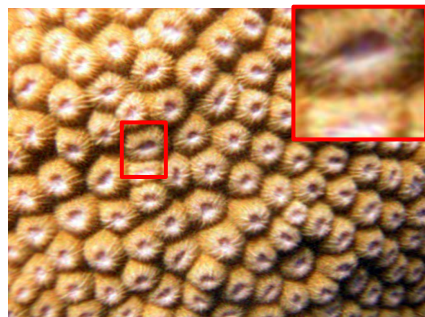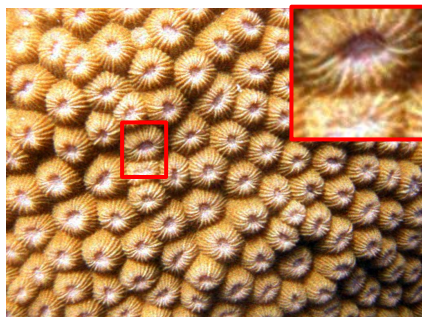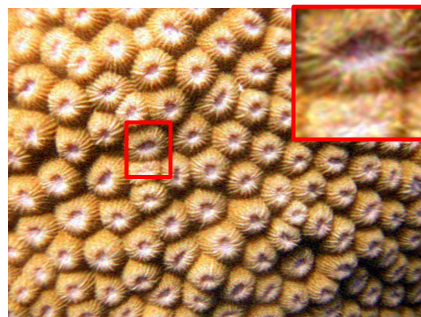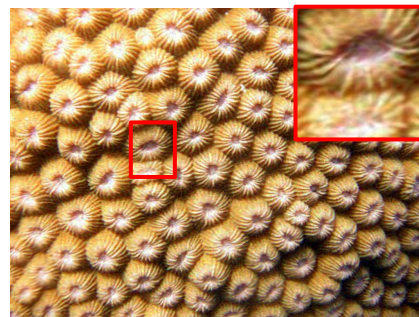

Gauss

Iterative-Gauss

WIRE

Iterative-WIRE



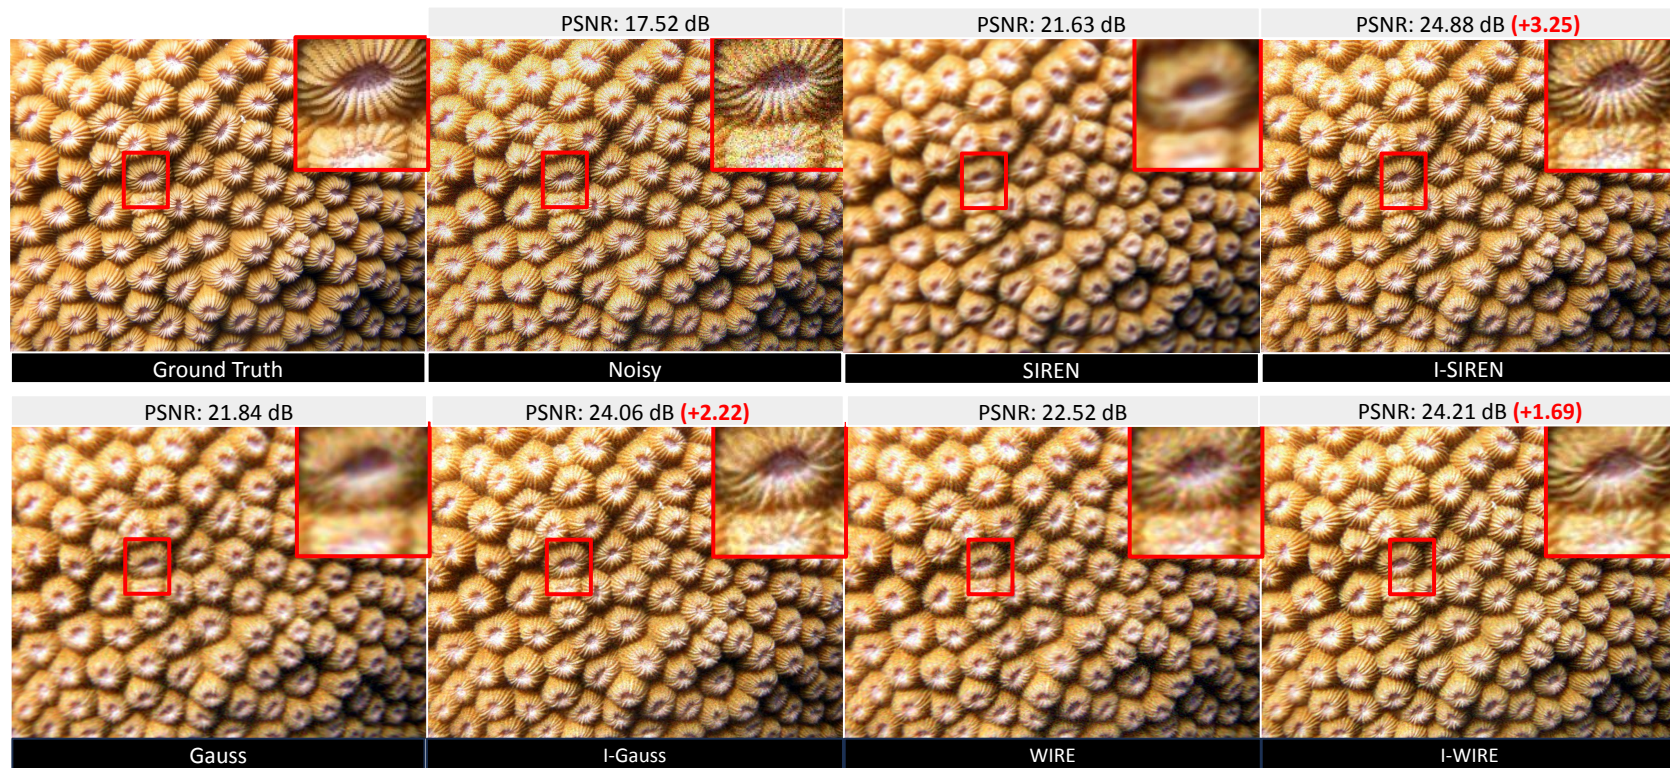

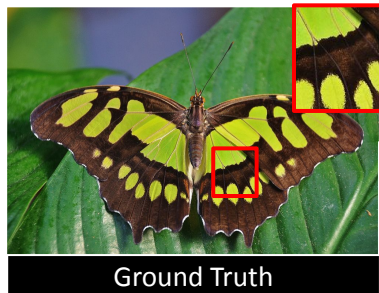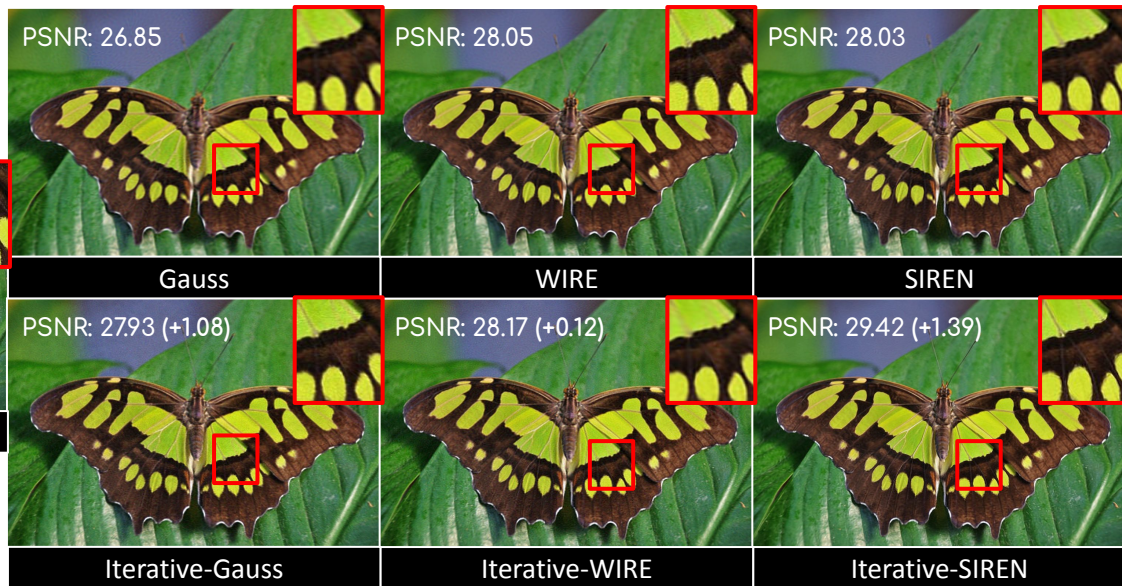



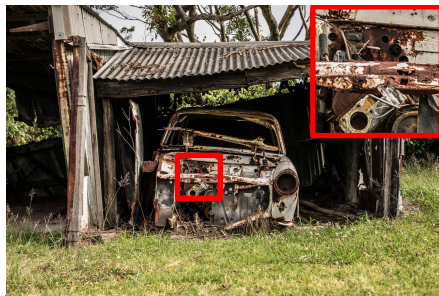

Ground Truth

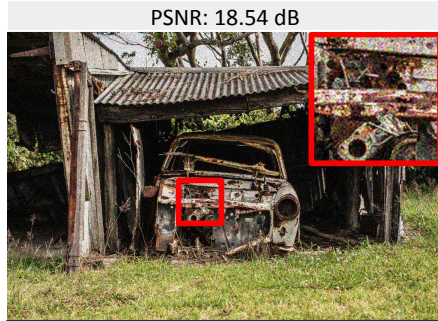

Noisy

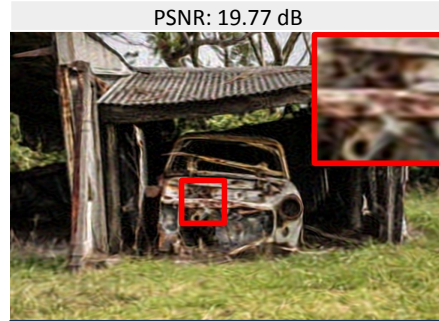

SIREN

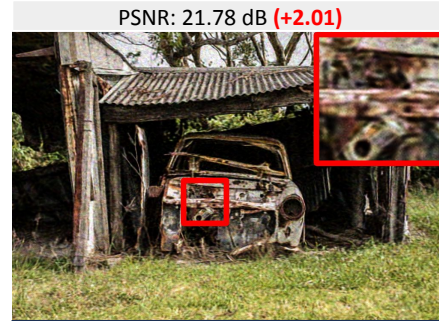

I-SIREN

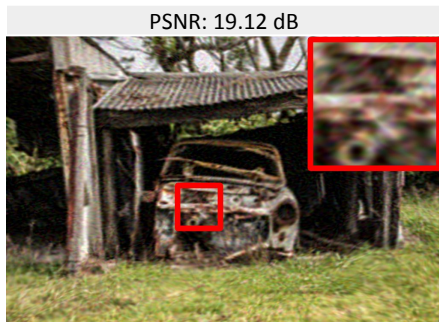

Gauss

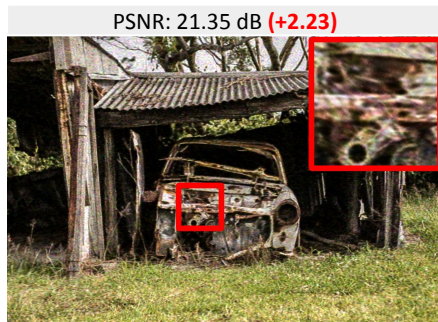

I-Gauss

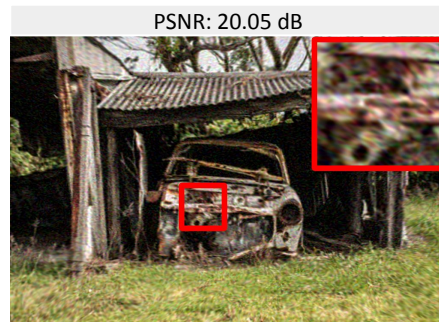

WIRE

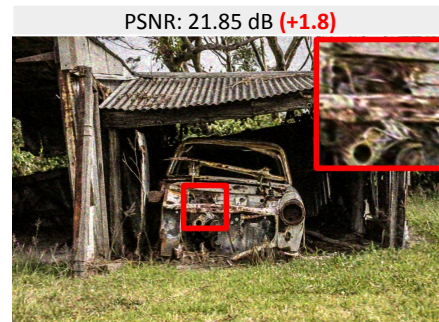

I-WIRE



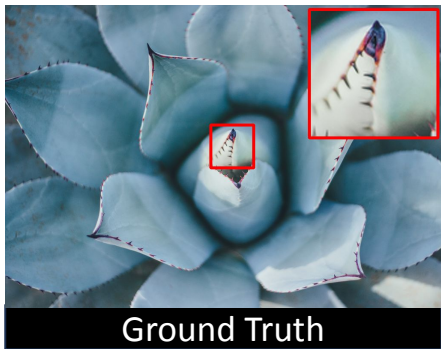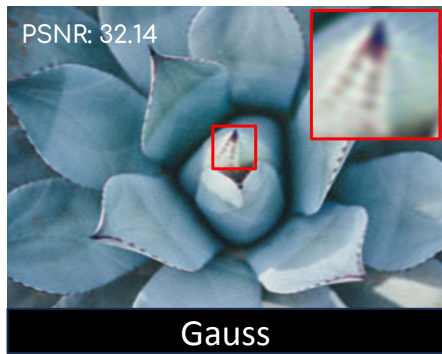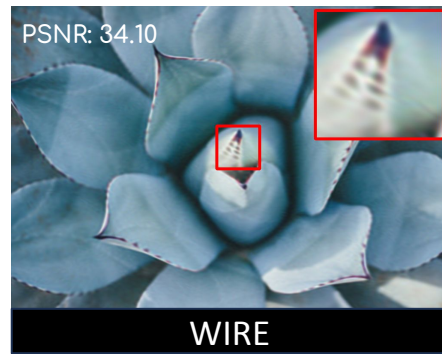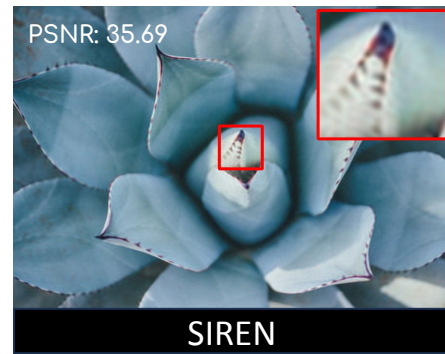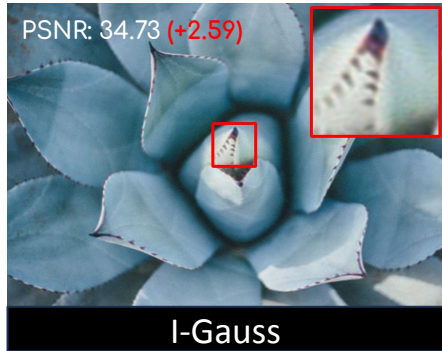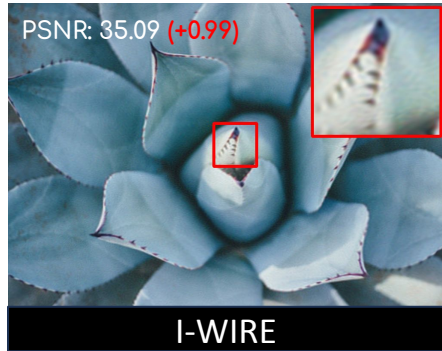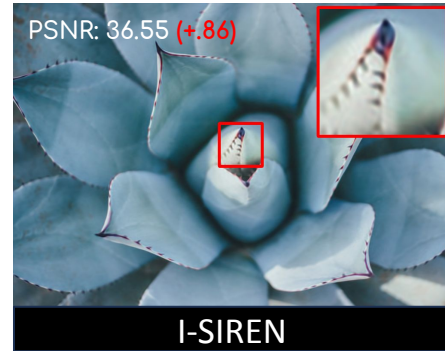

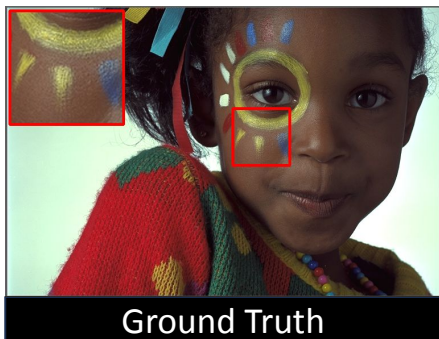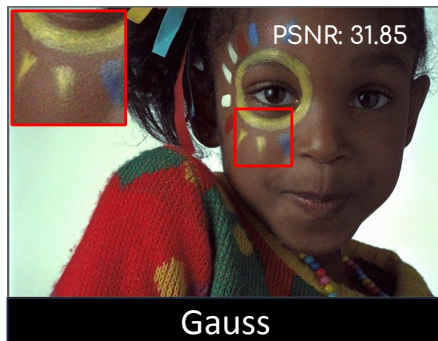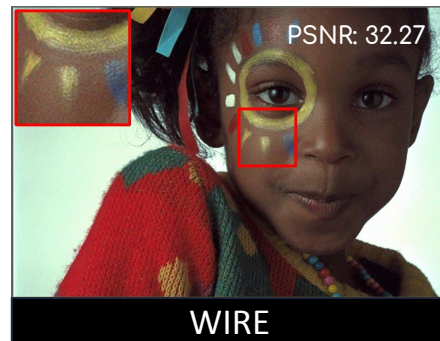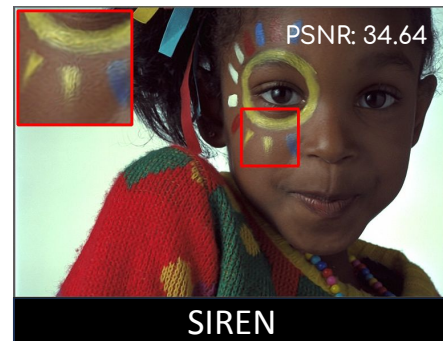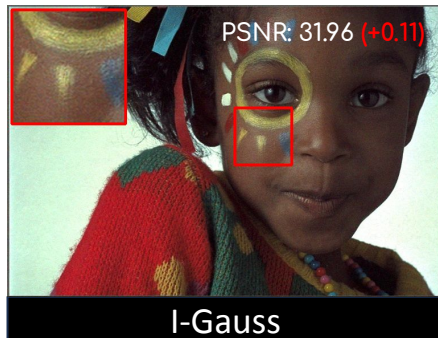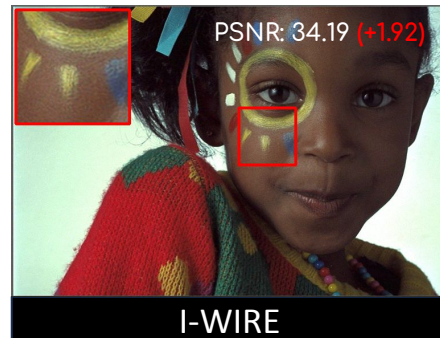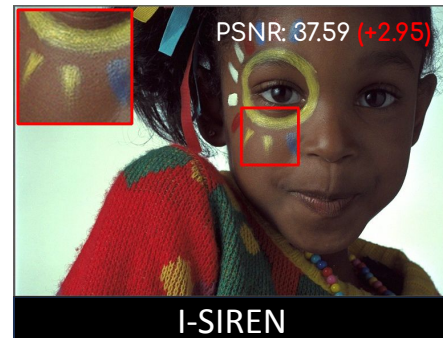



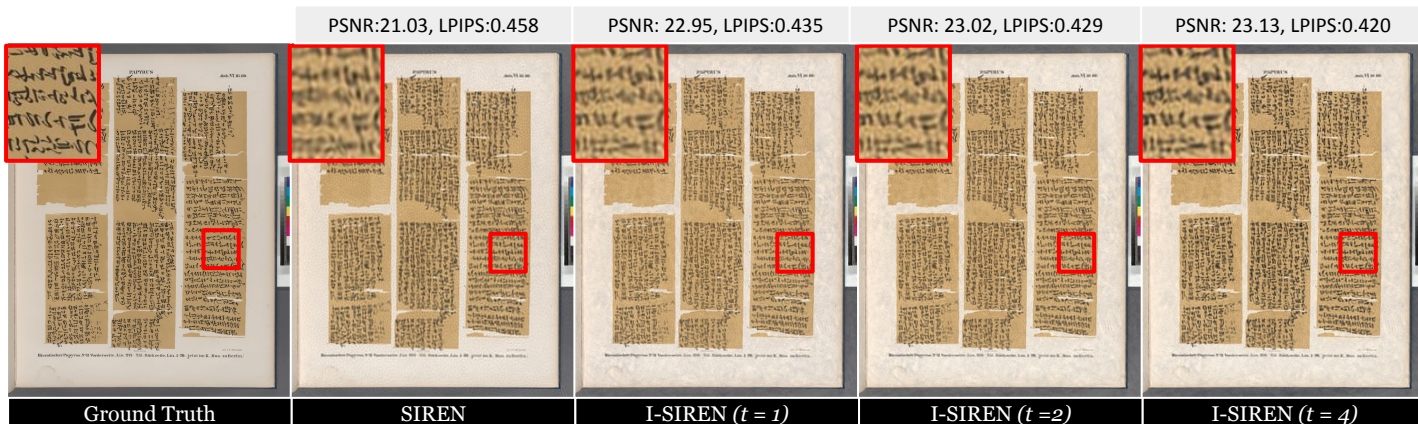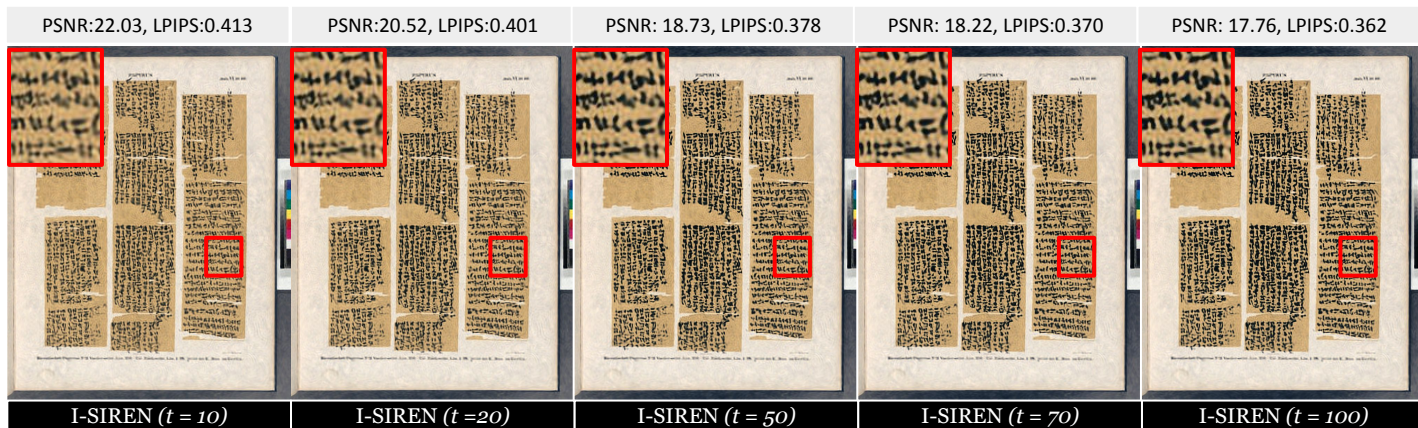

Supplement: Supplementary file 1 [file Supplementary_figs.pdf]
